# Supplementary material for: Morphological transitions of active Brownian particle aggregates on porous walls
Source: arXiv:2004.11436 ancillary file (2020-10-12)
Supplement: Supplementary file 1 [file Supplementary_Information.pdf]

# Morphological transitions of active Brownian particle aggregates on porous walls - Supplementary Information

Suchismita Das and Raghunath Chelakkot
*Department of Physics, Indian Institute of Technology Bombay, Mumbai - 400076, India*

## I. LIST OF SYMBOLS

| Parameter | Definition |
|---|---|
| $\mathbf{r}_i$ | Particle position |
| $\hat{\mathbf{e}}_i$ | Particle polarity |
| $\sigma$ | WCA interaction range |
| $\epsilon$ | WCA interaction strength |
| $D$ | Diffusion coefficient |
| $D_r$ | Rotational diffusion coefficient |
| $r_{ij}$ | Inter-particle distance |
| $Pe$ | Péclet number |
| $N$ | Number of particles |
| $\phi$ | Volume fraction |
| $\rho$ | Local density |
| $v_0$ | Particle motility |
| $\mu$ | Particle mobility |
| $\delta$ | Wall porosity |
| $h$ | Local height of the dense-phase |
| $\ell$ | Vacancy fraction |
| $N_c$ | Cluster fraction |
| $\|J_y\|$ | Absolute flux across the wall |
| $p_{\alpha\beta}^{s/I/w}$ | Pressure tensor components (swim/interaction/wall) |
| $p_N/p_T$ | Normal/ Tangential pressure component |
| $\gamma_{wl}$ | Wall-liquid interfacial tension |
| $\gamma_{lv}$ | Liquid-vapor interfacial tension |
| $S$ | Effective spreading parameter |

TABLE I. Table of parameters used.

## II. QUANTIFICATION OF DENSE-PHASE

### A. Cluster fraction

The fraction of total particles in the dense-phase (clusters) distinguishes between a phase-separated state and a homogeneous state. We consider two particles to be part of a cluster if they are within the interaction cutoff range, which is $2^{1/6}\sigma$ in this case. For all the parameter values which were analyzed, the bulk aggregation takes place near the wall. For a system size of $N = 9900$ active particles, we calculate the total number of particles which are part of the dense phase clustered around the wall $N_c$ and define cluster fraction as $N_c/N$, where $N$ is the total number of active particles in the system. We calculate this as a time-averaged quantity over steady states over 10 independent runs.

### B. Vacancy fraction

The vacancy fraction identifies different morphological states of the dense-phase. When the dense-phase is in CDP, the cluster covers the entire wall, while a portion of the length of the wall is free of aggregates, when the dense-phase form droplets. We can differentiate between the cluster morphology by computing the length of cluster-free space on the wall. We divide the system along the length of the wall into bins with a size equal to the particle diameter. If a particle is present in the bin, we consider it to be occupied. We can hence compute the total number of occupied bins, $n_{oc}$. Considering the total number of bins to be $n_{bin}$, the number of vacant bins will be $l_e = n_{bin} - n_{oc}$. The vacant fraction is then defined to be $\ell = l_e/L$. In CDP, the value of $\ell \simeq 0$, whereas for stable droplets, $\ell > 0.3$. However, near the transition point between CDP and droplets, $\ell$ incurs large fluctuations. Thus, we use $\ell = 0.1$ as a boundary between CDP and droplets.

### C. Interfacial length

For the connected clusters aggregating near the wall, we bin the system along its length along the x-axis, and for each bin, we locate the maximum $y$ coordinate, which we define as the local height $h(x)$. We calculate the difference in height between two adjacent bins, $h[j+1]-h[j]$, where $j$ runs over the bin index. Thus the length for each adjacent bin can be found as $([h[j+1]-h[j])^2+(x[j+1]-x[j])^2)^{1/2}$. This value can be summed over all the occupied bins to give an estimate of the length of the interface $L_{int} = \sum_{j=1}^{n_{oc}}([h[j+1]-h[j])^2 + (x[j+1]-x[j])^2)^{1/2}$. From Fig S1, we see a reduction in the interfacial length for the Disconnected Droplets by more than 30% when the cluster morphology changes from CDP to droplets.

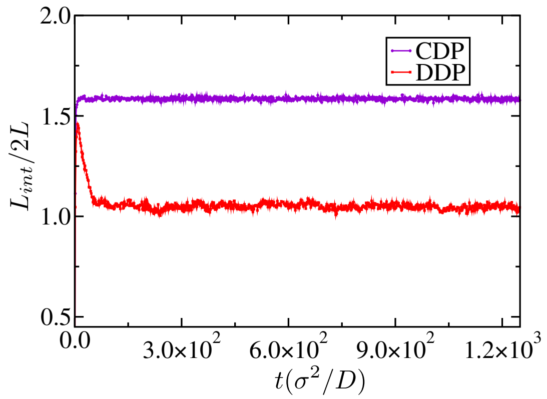


FIG. S1. Interface length as a function of time for CDP (violet) and droplet(red) states for $Pe = 200$, $N = 39800$ and $\delta = 1.85$, where we observe bistability. Disconnected droplets showing a clear reduction in interfacial length These were run over 40 realizations, with 14 cases showing droplets, while 26 cases formed connected dense phases. Here $L$ denotes the simulation box length.

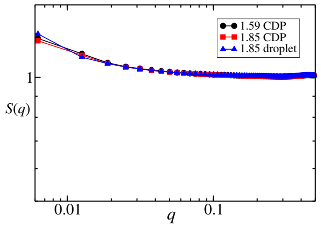


FIG. S2. The static structure factor $S(q)$ calculated for parameter values that provided different morphological states, $\delta = 1.59$, $Pe = 240$ (●), and $\delta = 1.85$, $Pe = 240$ (■) displaying CDP, and $\delta = 1.85$, $Pe = 240$ (▲) giving droplets.

### D. Structure factor

To further characterize the clustering behaviour, we have calculated the static structure factor $S(q)$ for different parameters, corresponding to both CDP and droplet states. The $S(q)$ vs. $q$ provides similar pattern for all the three cases (Fig S2). Also, the typical scaling for bulk MIPS is absent in $S(q)$. The pattern $S(q)$ is similar to the profile obtained for low $\phi$ in other studies [1, 2].

## III. DEPENDENCE OF CLUSTERING BEHAVIOR ON SYSTEM SIZE

We analyze the dense-phase formation on the porous walls at different system sizes, defined by the number of ABPs for a fixed value of their area fraction, $\phi$. We examine the dense-phase formation with $N = 2450, 5112, 9900, 39800, 89700, 159600$, and $N = 249500$ and had observed distinct morphological transitions in all these systems. The dense-phase morphology is quantitatively identified using the vacancy fraction $\ell$, as described in the previous section. We analyze the time evolution of $\ell$ for three sets of parameters corresponding to different morphological states.

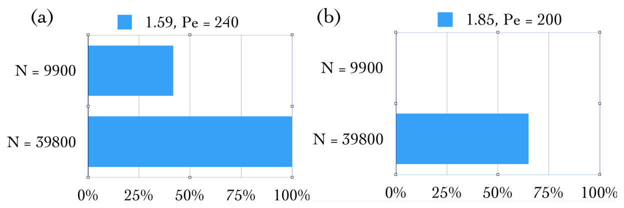


FIG. S3. We analyze what fraction of independent simulations form CDP (a) For separation 1.59, $Pe = 240$, we find 50 out of 120 independent runs form continuous clusters in case of $N = 9900$ active particles, whereas all 40 independent runs form continuous clusters in case of $N = 39800$ active particles. (b) For separation 1.85, $Pe = 200$, 0 out of 40 independent runs form continuous clusters in case of $N = 9900$ active particles, whereas 26 out of 40 independent runs form continuous clusters in case of $N = 39800$ active particles.

### A. Bistability

We observe the morphological transition from CDP to droplets for all the system sizes. However, the transition point and the parameter region where we observe bistability, depends on the system size. For example, in Fig S3, $\delta = 1.59$, $Pe = 240$ is a bistable parameter for $N = 9900$, but it is in Connected Dense Phase for $N = 39800$. Again, while $\delta = 1.85$, $Pe = 200$ shows a droplet phase for $N = 9900$, it is bistable for $N = 39800$. We thus note that this feature of bistability is observed in different system sizes, though with a parametric shift.

### B. Connected Dense Phase

We study the finite size dependence for a system which shows Connected Dense Phase clusters for all independent runs. To test whether the clusters remain as CDP, we simulate for the different system sizes mentioned previously and note that it shows no transitions to droplets whatsoever. In Fig S4, we plot the vacancy fraction as a function of time for $\delta = 1.59$, $Pe = 120$. After a short transient time ($t < 10$), $\ell$ saturates at a small value for all system sizes.

#### 1. *Effect of lowering density*

We have also studied the effect of lowering particle density for narrow pores. In this paper, we have kept the particle density constant at 0.3. We have seen the effect

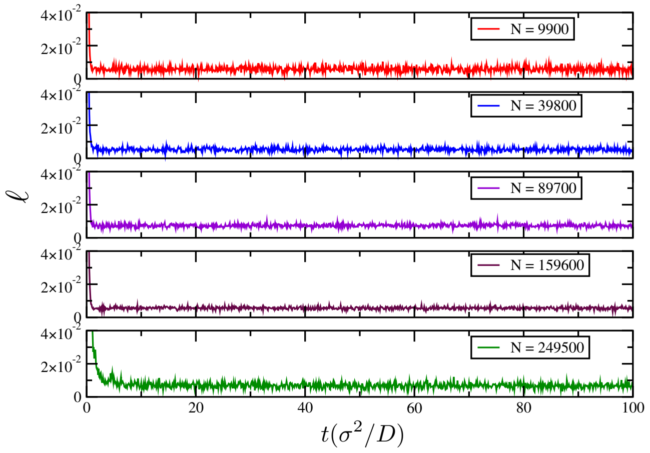


FIG. S4. Testing the finite size dependence of systems which remain as CDP for all independent runs. We plot the vacancy fraction, $\ell$, as a function of time for system sizes $N = 9900, 39800, 89700, 159600$ and $N = 249500$, averaged over several independent runs. For all the system sizes, $\ell$ saturates around $\ell \simeq 0.01$ after a short transient time. This was done for $\delta = 1.59$, $Pe = 120$, averaged over multiple independent runs. For $N = 9900, 39800, 89700$ and $159600$, the simulations were over 10 independent runs, while $N = 249500$, the simulations are over 2 independent runs.

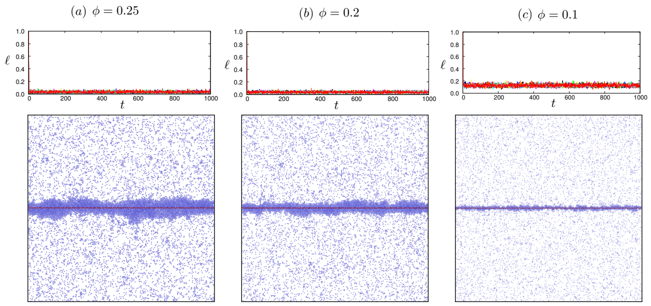


FIG. S5. Effect of lowering density (a) $\phi = 0.25$, (b) $\phi = 0.2$, (c) $\phi = 0.1$ for $\delta = 1.25$ and $Pe = 150$. This was done for $N = 9900$ active particles for 10 independent runs.

of lowering density for $\phi = 0.25$, $\phi = 0.2$ and $\phi = 0.1$, keeping the porosity fixed at $\delta = 1.25$ and activity at $Pe = 150$ for $N = 9900$ active particles for 10 independent runs. We indeed see that connected dense phase is the only option for narrow pores (as can be seen from Fig S5), with the wall interaction studied in this paper. When $\phi \leq 0.1$, the clustering behaviour starts to disappear.

## C. Disconnected Droplets

We also study the finite size dependence for systems showing Disconnected Droplet state at $\delta = 1.85$ and $Pe = 240$ (Fig S6). For $N = 9900$ and $N = 39800$, we run the simulation for $t > 1000$ and clearly see that

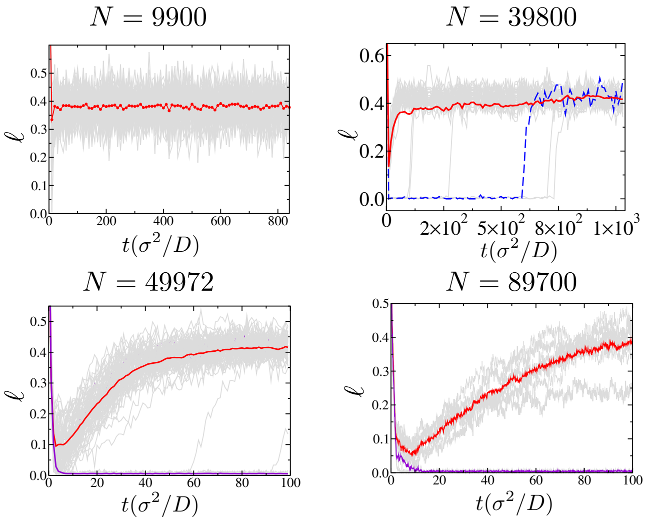


FIG. S6. Testing the finite size dependence of systems that prefer droplets. We plot the vacancy fraction as a function of time for system sizes $N = 9900, 39800, 49972$ and $89700$. The grey lines indicate independent trajectories. The red line is averaged over the runs, which form droplets; the violet line is averaged over the runs, which form CDP. The blue line in $N = 39800$ indicates a typical transitioning trajectory from CDP to droplets. This was done for $\delta = 1.85$ and $Pe = 240$, averaged over multiple independent runs.

all the independent runs form a droplet. We also find a few state form droplets at a later stage in the simulation for $N = 39800$, as evident from the abrupt jump in $\ell$ from zero to a larger value. For even larger systems with $N = 49972, 89700, 159600$ and $N = 249500$, the runs are relatively shorter ($t = 100$) due to computational limitations. However, these runs also show a clear trend of preferring droplets over CDP, with $\ell$ converging to a non-zero value. The number of independent runs for the system sizes are 80 for $N = 9900$, 40 for $N = 39800$, 120 for $N = 49972$, 10 for $N = 89700$ and $N = 159600$ and 5 for 249500. All the independent runs for $N = 9900$ and $N = 39800$ converge to droplets. For other system sizes, we observe that 79 out of 120 independent runs ($N = 49972$), 7 out 10 independent runs ($N = 89700$ and $N = 159600$) and 4 out of 5 independent runs ($N = 249500$) prefer droplets till ($t = 100$), with some late-time transitions happening from CDP to droplets. We expect this trend to continue until all the runs converge at longer times. For $N = 159600$ and $N = 249500$, though we do observe a preference to form droplets, the saturation time is greater than the run time and hence we do not plot it here.

### 1. *Dependence of system size near boundary of Connected Dense Phase and Disconnected Droplets*

From our analysis of varying wall porosity with activity, we find that for a system size of $N = 9900$, we do not

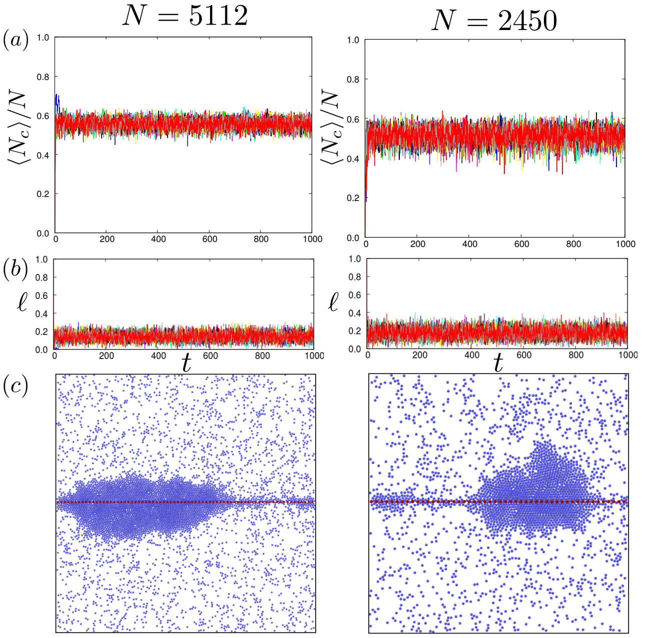


FIG. S7. (a) Cluster fraction $\langle N_c \rangle / N$, (b) empty space fraction $\ell$ as a function of time and (c) snapshots for $N = 5112$ and $N = 2450$ active particles for $\delta = 1.59$, $Pe = 240$, showing emergence of droplets for lower system sizes near boundary. This was done for 10 independent runs.

observe formation of droplets for $\delta < 1.59$. At $\delta = 1.59$, we observe bistability at $Pe \geq 190$. We study the system size dependence in the clustering behaviour at this boundary value ($\delta = 1.59$), for high motility ($Pe = 240$), where we observe bi-stable clusters for $N = 9900$. However, for larger system size ($N = 39800$), the bistable behaviour disappears and we observe only CDP. Whereas for lower the system size ($N = 5112$ and $N = 2450$), droplets are formed for these parameters (Fig S7). But, for a smaller pore-size ($\delta = 1.25$), where we observe CDP at $N = 9900$, the clustering behaviour does not get affected by the change in system size S8. We observe the formation of CDP for $N = 2450$, $N = 5112$, $N = 9900$, and $N = 39800$ for all the 10 independent runs.

We also test the effect of lowering system size for a parameter known to form stable droplets for $N = 9900$ and $N = 39800$ ($\delta = 1.85$, $Pe = 240$). We find that the droplets survive for $N = 5112$ and $N = 2450$ for 10 independent runs. However, fluctuations start becoming very high for $N = 2450$, with gradual appearance and disappearance of droplets as can be seen in Fig S9.

## IV. COARSENING

We study whether the cluster geometry gets affected by the coarsening of dense-phase, which has been observed in previous studies on MIPS. For its quantification, we plot the fraction of the largest cluster ($N_c/N$) as a function of time in Fig S10 for both morphological

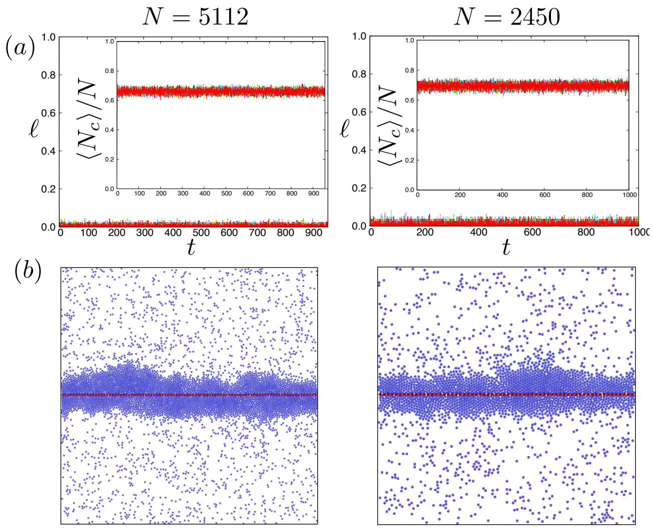


FIG. S8. (a) Empty space fraction $\ell$ and (inset) cluster fraction $\langle N_c \rangle / N$, as a function of time, (b) snapshots for $N = 5112$ and $N = 2450$ active particles for $\delta = 1.25$, $Pe = 240$, showing stability of connected dense phase morphology for a narrow pore. This was done for 10 independent runs.

states. We find that though it increases steeply in the nucleation stage till $t \simeq 10$, the dense-phase fraction is saturated at late times. In this case, the aggregate clearly prefers a droplet geometry for high porosity and high activity. The saturated value $N_c/N$ is marginally smaller for the droplet state. We also find an abrupt decrease in $N_c$ when the morphology changes from CDP to droplets.

## V. CALCULATION OF PRESSURE AND SURFACE TENSION

To closely analyze the mechanical properties of the dense-phase, we calculate the spatial variation of pressure as a function of distance from the wall. We decompose the space into $n_b$ bins parallel to the wall, such that its width $\delta y = L/n_b$, where $L$ is the system size. The contribution to pressure due to particle interaction can be calculated directly as

$$p^I_{\alpha\beta}(y) = \frac{1}{2L\delta_y} \langle \sum_{(i/j)\in\delta_y} F_{ij\alpha} r_{ij\beta} \rangle_T, \qquad (1)$$

where $r_{ij} = r_i - r_j$ is the distance between the $i$-th and $j$-th particles, and $F_{ij}$ is the interaction force due to WCA potential between them[3, 4]. $\langle . \rangle_T$ denotes the time average. $\alpha$ and $\beta$ denote the Cartesian indices.

The second part to the pressure contribution stems from the activity of the particles. These particles can be thought of exerting an 'impulse' $\boldsymbol{j}_i$, which is governed by its self-propulsion force $F_p = v_0/\mu$ directed along the

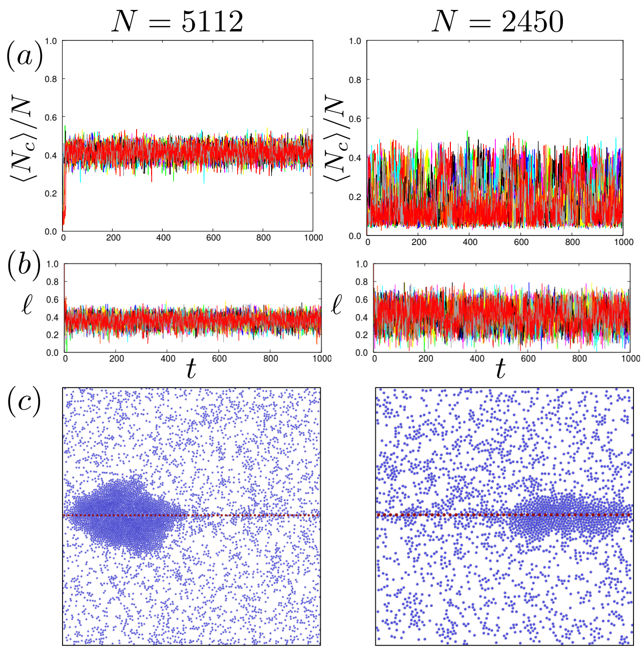


FIG. S9. (a) Cluster fraction $\langle N_c \rangle / N$, (b) empty space fraction $\ell$ as a function of time and (c) snapshots for $N = 5112$ and $N = 2450$ active particles for $\delta = 1.85$, $Pe = 240$. This was done for 10 independent runs.

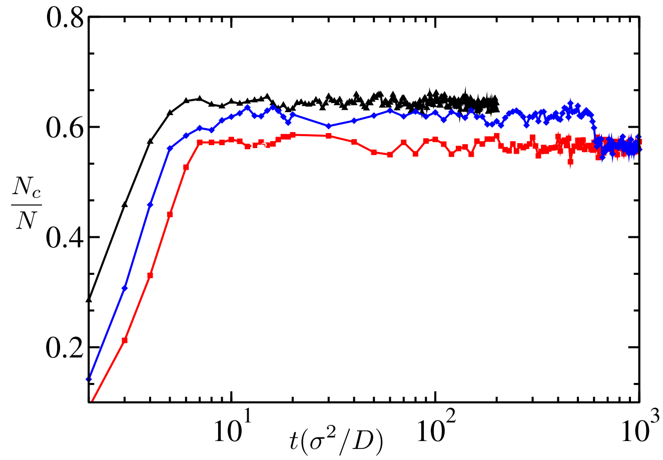


FIG. S10. Largest cluster fraction as a function of time for three typical trajectories. Here CDP corresponds to $\delta = 1.59$, $Pe = 240$ (shown here till $t = 200$ in black), and DDP (in red) as well as transition from CDP to DDP (in blue) corresponds to $\delta = 1.85$, $Pe = 240$. Though initially there is a steep increase, the largest cluster fraction shows a steady behavior beyond ($t \geq 10$). This was done for $N = 39800$.

orientation vector $\hat{\mathbf{e}}_i$ over a time scale determined by its rotational diffusion $1/D_r$, $\boldsymbol{j}_i = F_p \hat{\mathbf{e}}_i / D_r$ [5]. The swim pressure then can be computed as

$$p^s_{\alpha\beta}(y) = \frac{1}{2L\delta_y} \langle \sum_{i \in \delta_y} j_{i\alpha} v_{i\beta} \rangle_T, \tag{2}$$

where $\mathbf{v}_i$ is the velocity of the $i$-th particle. Finally the pressure resulting from the interaction with the wall particles contribute only till the interaction cutoff range with the wall, that is within a distance of $2^{1/6}\sigma$. This can be formulated as

$$p^w_{\alpha\beta}(y) = \frac{1}{L\delta_y} \langle \sum_i F_{iw\alpha} r_{iw\beta} \rangle_T, \tag{3}$$

where $F_{iw}$ is the interaction force of the wall particles with the active particles and $r_{iw}$ is the distance of the $i$-th active particle with the $w$-th wall particle. We have kept $\delta y = 2^{(1/6)}\sigma$ in the analysis. Because of the wall porosity, the particles can be found in between two 'wall' particles at a given time, which contributes to a tangential component of pressure, unlike the case of impenetrable walls. For a given surface, the total interfacial tension can be calculated using the mechanical relation [6],

$$\gamma_{\text{tot}} = \int_{-L/2}^{L/2} (p_N - p_T) dy \tag{4}$$

, where $p_N$ and $p_T$ are the pressure components which are normal and tangential to the interface.

### A. In presence of porous walls

When the dense-phase forms CDP, the interface is on an average parallel to the wall. One can approximate $\hat{\mathbf{e}}_x$ to be parallel to the interface and $\hat{\mathbf{e}}_y$ to be normal to the interface. In Fig S11 and S12, the pressure contribution arising from interaction, swim and wall have been shown separately for $\delta = 1.59$ , $Pe = 240$ and $\delta = 1.85$ and $Pe = 240$ respectively for $N = 39800$ active particles. In case of $\delta = 1.85$, we have analysed over 18 independent runs (123008 configurations) maximum till time $200\tau$ for configurations which remain as connected clusters, while for $\delta = 1.59$, we have analysed over 40 independent runs (60040 configurations, time $200\tau$). The normal component of the total pressure is continuous across the CDP - bulk interface, as verified by previous studies. We have also checked that the normal pressure has a constant value at the interface and bulk.

To compare the orientation along the normal component, we plot it for two different cases in Fig S13, having pore sizes $\delta = 1.59$ and $\delta = 1.85$, each having $Pe = 120$ and $Pe = 240$. For $\delta = 1.59$, $Pe = 240$, we have connected dense phases quite early. For the larger pore size, the transient states are longer. We see that for $\delta = 1.59$, there is no preferred alignment for the active particles near the wall, whereas for $\delta = 1.85, Pe = 240$, there seems to be weak alignment close to the wall, with

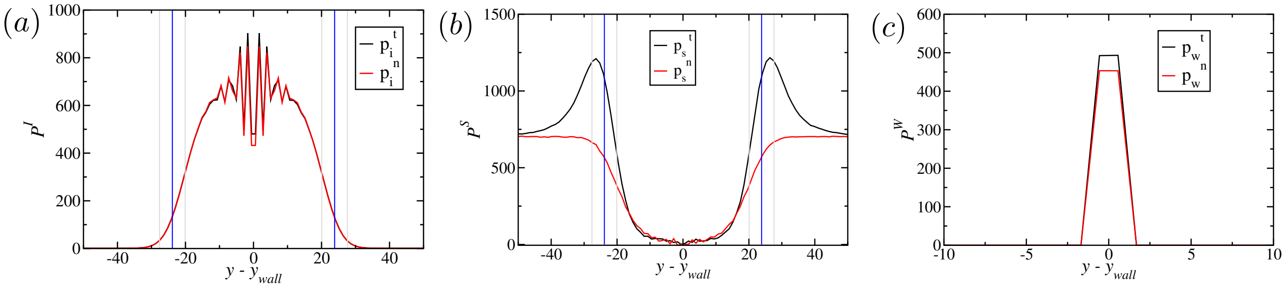


FIG. S11. N = 39800, $\delta = 1.59$, Pe = 240, 40 runs, 60040 configurations, $\langle h \rangle = 23.86$ (blue line), $(\langle h^2 \rangle - \langle h \rangle^2)^{1/2} = 3.77$ (grey line) (a) Interaction pressure versus distance from wall. (b) Swim pressure versus distance from wall. (c) Pressure due to wall interaction versus distance from wall.

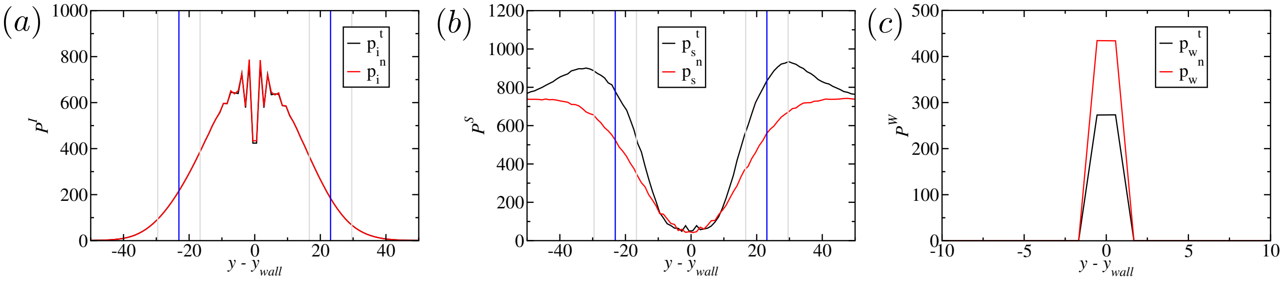


FIG. S12. N = 39800, $\delta = 1.85$, Pe = 240, 18 runs (continuous), 123008 configurations, $\langle h \rangle = 23.11$ (blue line), $(\langle h^2 \rangle - \langle h \rangle^2)^{1/2}$ = 6.46 (grey line) (a) Interaction pressure versus distance from wall. (b) Swim pressure versus distance from wall. (c) Wall pressure versus distance from wall.

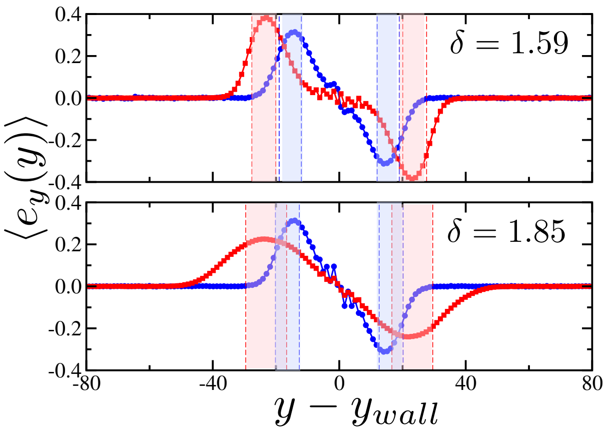


FIG. S13. Orientation along normal direction for the case of porous walls for $Pe = 120$ (blue), $Pe = 240$ (red), (a) $\delta = 1.59$, and (b) $\delta = 1.85$ as a function of distance from wall.

broader interfacial width.

We tabulate the values of the wall-liquid tension $\gamma_{wl}$ for $\delta = 1.85$ and $\delta = 1.59$ in Table II and III. Here $n*$ denotes the number of steady-state configurations analysed. As shown in Table II, the value of $\gamma_{wl}$ steadily increases with $Pe$. This behaviour is consistent with the higher tendency to form droplets on the wall. However, when an

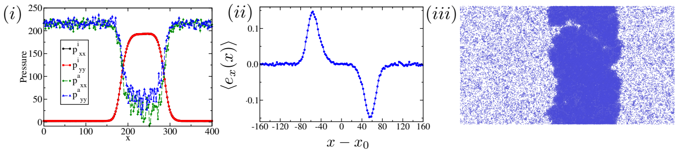


FIG. S14. (i) Interaction pressure and swim pressure generated for a similar system as in [3]. (ii) Orientation along normal direction for the case without walls for a slab geometry having $Pe = 100$ and packing fraction 0.5 with slab aligned along $y$ axis. Here $x_0$ denotes the approximate midpoint of the cluster. (iii) Snapshot of simulation of system as in [3], with $L_x = 402$ and $L_y = 202$ with $N = 52325$ active particles.

effective spreading parameter $S = -(\gamma_{wl} + \gamma_{lv})$ is calculated by adding the contribution from the liquid-vapour interfacial contribution, we do not observe a consistent increase in $S$ with the tendency to form CDP.

## B. MIPS in absence of wall

We have also studied the system without introducing porous walls for verification, with similar conditions as in [3]. We analyse the system having slab geometry, using packing fraction 0.5 and $Pe = 100$ in a rectangular box with $N = 52325$ active particles. We choose a rectangular box of size $L_x = 402$ and $L_y = 202$. The rectangular geometry of the simulation box facilitates a slab-like ge-

| Activity | Pe = 240 | Pe = 200 | Pe = 160 | Pe = 120 |
|---|---|---|---|---|
| $\gamma_{WL}$ | 237 | 224 | 184 | 129 |
| $\gamma_{LV}$ | -6578 | -4015 | -2188 | -975 |
| $S$ | 6341 | 3791 | 2004 | 846 |
| $n*$ | 123008 | 3576 | 4760 | 5960 |

TABLE II. Interfacial tension values for the wall-liquid interface $\gamma_{wl}$, the liquid-vapour interface $\gamma_{lv}$, and the effective spreading parameter $S = -(\gamma_{lv}+\gamma_{wl})$ for $\delta = 1.85$, $N = 39800$ active particles.

| Activity | Pe = 240 | Pe = 120 |
|---|---|---|
| $\gamma_{WL}$ | -208 | 131 |
| $\gamma_{LV}$ | -7066 | -929 |
| $S$ | 7274 | 798 |
| $n*$ | 60040 | 11920 |

TABLE III. Surface tension values for $\delta = 1.59$, $N = 39800$ active particles.

ometry for the dense-phase. We also get similar pressure profiles, confirming the behavior obtained in [3]. Further, we have also analysed the orientation of the active particles in the condensed dense phase, as shown in Fig S14. We do not find any preferred alignment for the active particles inside the connected dense phase, though in case of porous walls even with high porosity ($\delta = 1.85$), there is a non-zero mean alignment in the dense-phase (Fig S13).

## VI. CONTACT ANGLE ANALYSIS

In our analysis, we calculate $\gamma_{wl}$ and $\gamma_{lv}$ for parameters where the CDP is stable and where the CDP is unstable and forms droplets at later times. When the CDP transforms into droplets, another interface (wall-vapour) appears. In such cases, we perform the integration given in Eq.(5) of the main text for the part of wall where the dense region is not present. This integration provides the wall-vapour interfacial tension $\gamma_{wv}$. We find that the interaction pressure and the wall pressure are negligible, whereas swim pressure contribution is higher for $\gamma_{wv}$. We conduct our analysis for $\delta = 1.85$ in case of $N = 39800$ particles for $Pe = 200$ and $Pe = 240$. We choose 4 independent runs which form droplets for estimating the value of wall-vapour interfacial tension (Fig. S15), tabulated in Table IV. Since these values are sensitive to swim pressure contribution, we obtain large variations in $\gamma_{wv}$ across independent runs. After the aggregate form steady droplets, we calculate the time-averaged density profile(Fig. S16) and obtain the averaged boundary of the dense region. This allows us to calculate the contact angle ($\theta_c$) that the droplet makes with the wall. We compare this computed $\theta_c$ to the contact angle predicted by Young's equation, $\cos\theta_c = (\gamma_{wv}-\gamma_{wl})/\gamma_{lv}$ (given in Table IV). Our calculations indicate that Young's equation for wetting liquids in equilibrium is not valid for measured $\gamma$ values.

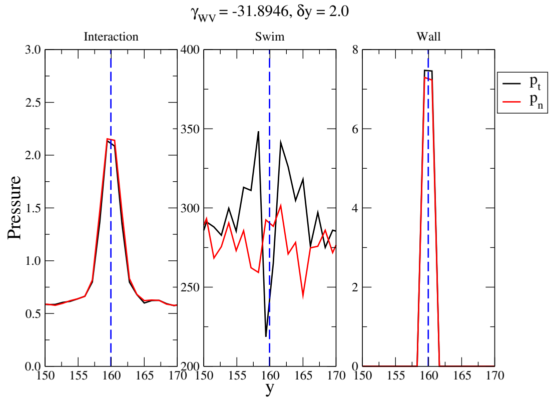


FIG. S15. Estimating the value of solid-vapor interfacial tension for $N = 39800$ active particles, $\delta = 1.85$ and $Pe = 200$ for 4 independent runs which form droplets.

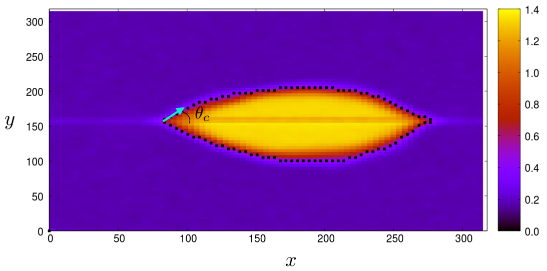


FIG. S16. Time-averaged local density for a droplet configuration from which we estimate the contact angle. This was done for $N = 39800$ active particles for $\delta = 1.85$ and $Pe = 200$.

| Activity | $Pe = 240$ | $Pe = 200$ |
|---|---|---|
| $\gamma_{WL}$ | 237 | 224 |
| $\gamma_{LV}$ | $-6578$ | $-4015$ |
| $\gamma_{WV}$ | $-87$ | $-32$ |
| $\theta_c$ measured (in °) | 51.9 | 40.4 |
| $\theta_c$ calculated (in °) | 87.2 | 86.4 |

TABLE IV. Estimating values of contact angle (from 4 independent droplet configuration) and surface tension for $\delta = 1.85$ and $N = 39800$. The third row denotes the contact angles directly measured from the simulation. The fourth row provides the contact angle calculated from Young's law, $\theta_c = \arccos\{(\gamma_{wv} - \gamma_{lv})/\gamma_{wl}\}$.

## VII. MOVIES

Movies have been generated using the OVITO software[7].
Movie 1: Formation of connected dense phase. Corresponds to Fig 1(a) of main text.
Movie 2: Formation of disconnected droplets. Corresponds to Fig 1(b) of main text.
Movie 3: Transition of connected dense phase to disconnected droplets. Corresponds to Fig 1(c) of main text.
Movie 4: Transition of disconnected droplets to connected dense phase. Corresponds to Fig 1(d) of main text.
Movie 5: Cluster stability in presence of nucleation seeds. Corresponds to Fig 3(a) of main text.
Movie 6: Cluster reversibility by changing activity. Corresponds to Fig 3(b) of main text.


[1] Y. Fily and M. C. Marchetti, *Phys. Rev. Lett.*, 2012, **108**, 235702.

[2] Q.-L. Lei, M. P. Ciamarra and R. Ni, *Science advances*, 2019, **5**, eaau7423.

[3] J. Bialké, J. T. Siebert, H. Löwen and T. Speck, *Phys. Rev. Lett.*, 2015, **115**, 098301.

[4] A. E. Patch, *PhD thesis*, 2018.

[5] Y. Fily, Y. Kafri, A. P. Solon, J. Tailleur and A. Turner, *Journal of Physics A: Mathematical and Theoretical*, 2017, **51**, 044003.

[6] J. G. Kirkwood and F. P. Buff, *The Journal of Chemical Physics*, 1949, **17**, 338–343.

[7] A. Stukowski, *Modelling and Simulation in Materials Science and Engineering*, 2010, **18**, 015012.
